# Supplementary material for: Stable Adversarial Learning under Distributional Shifts
Source: arXiv:2006.04414 source file (2021-05-11)
Supplement: Supplementary file 1 [file appendix.tex]

\appendix

\section{Related Work}
\subsection{Robust Learning} 
Recently, robust learning methods including adversarially robust\cite{papernot2016limitations,madry2017towards,ye2018bayesian} and distributionally robust algorithms\cite{SinhaCertifying, esfahani2018data,duchi2018learning} has been a research hotspot. 
While these methods provide robustness guarantees, they aim at subtle perturbations and cannot effectively achieve uniformly good performance under arbitrary distributional shifts. 
Furthermore, they equally treat all covariates when building the uncertainty set, which to some extent results in the over-pessimism problem for they optimize for implausible worst-case scenarios\cite{frogner2019incorporating}.

\subsection{Wasserstein Distance in Machine Learning}
Wasserstein distance arouses more and more attentions in machine learning community. WGAN\cite{pmlr-v70-arjovsky17a} replace the original JSD in the framework of GAN with Wasserstein distance and achieves better performance. \cite{DBLP:conf/nips/FrognerZMAP15} uses Wasserstein distance to measure the dissimilarity of the prediction and the target label for multi-label learning. In this work, we consider the distributional robustness over a distribution set which is formed by Wasserstein distance.

\section{Pseudo-code of SAL}
The pseudo-code of the whole Stable Adversarial Learning (SAL) algorithm is shown in algorithm \ref{algo:SAL}. 

\begin{algorithm}[]
  \caption{Stable Adversarial Algorithm}
  \label{algo:SAL}
\begin{algorithmic}
  \STATE {\bfseries Input:} Multi-environments data $D^{e_1},\ D^{e_2},\ \dots,\ D^{e_n}$, where $D^e=(X^e,Y^e)$, $e\in \mathcal{E}$
  \STATE {\bfseries Hyperparameters:} $T$, $T_{\theta}$, $T_w$, m,  $\epsilon_x$, $\epsilon_{\theta}$, $\epsilon_w$, $\alpha$
  \STATE {\bfseries Initialize:} $w = [1.0, \dots, 1.0]$
  \FOR{ $i=1$ {\bfseries to} $T$}
  
        \FOR{$j=0$ {\bfseries to} $T_{\theta}-1$}
            \STATE Initialize $\hat{X}_0$ as: $\hat{X}_0 = X$
            \FOR{$k=0$ {\bfseries to} $m-1$}
                \STATE
                \algorithmiccomment{Approximate the supreme of $s_{\lambda}(X)$ for $X^e$ from all $e\in\mathcal{E}$}
                
                \STATE $\hat{X^e}_{k+1} = \hat{X^e}_{k} + \epsilon_x\nabla_x\{\ell(\theta;\hat{X^e}_{k}) - \lambda c_w(\hat{X^e}_{k},\hat{X}_0)\}$

            \ENDFOR
            
            \STATE {\bf Update $\theta$ as:\ \ } $\theta^{j+1} = \theta^{j} - \epsilon_{\theta}\nabla_{\theta} \ell(\theta^j;(\hat{x}^m,y))$
        \ENDFOR
        
        \STATE {\bf Calculate $R(\theta)$ as:\ \ }$R(\theta)=\frac{1}{|\mathcal{E}|}\sum_{e\in\mathcal{E}}\mathcal{L}^e + \alpha\left(\sup\limits_{p,q\in \mathcal{E}}\mathcal{L}^p - \mathcal{L}^q\right)$
        
        \STATE $w^0 = w^{i}$
        \FOR{$j=0$ {\bfseries to} $T_w-1$}
            \STATE {\bf Update $w$ as:\ \ }$w^{j+1}=w^j - \epsilon_w\nabla_wR(\theta)$
        \ENDFOR
        \STATE {\bfseries Update w as:\ \ }, $w^{i+1}=\mathop{Proj}_{\mathcal{W}}\left(w^{t_w}\right)$.
  \ENDFOR
\end{algorithmic}
\end{algorithm}

\section{Deduction of $\ \partial R/\partial w$}
Here we provide the detailed deduction of $\partial R(\theta(w))/\partial w$, which can be approximated as following. 
\begin{equation}
	\frac{\partial R(\theta(w))}{\partial w} = \frac{\partial R}{\partial \theta}\frac{\partial \theta}{\partial X_A}\frac{\partial X_A}{\partial w}
\end{equation}
The first term $\partial R/ \partial \theta$ can be calculated easily.
The second term can be approximated during the gradient descent process of $\theta$ as :
\begin{align}
	\theta^{t+1} &= \theta^t - \epsilon_{\theta}\nabla_{\theta}\hat{\mathcal{L}}(\theta^t;X_A,Y)\\
	\frac{\partial \theta^{t+1}}{\partial X_A} &= \frac{\partial \theta^{t}}{\partial X_A} - \epsilon\frac{\nabla_{\theta}\hat{\mathcal{L}}(\theta^t;X_A,Y)}{\partial X_A}\\
	\frac{\partial \theta}{\partial X_A} &\approx -\epsilon\sum_t \frac{\nabla_{\theta}\hat{\mathcal{L}}(\theta^t;X_A,Y)}{\partial X_A}
\end{align}
where $\frac{\nabla_{\theta}\hat{\mathcal{L}}(\theta^t;X_A,Y)}{\partial X_A}$ can be calculated during the training process. The third term $\partial X_A / \partial w$ can be approximated during the adversarial learning process of $X_A$ as:
\begin{align}
	X_A^{t+1} &= X_A^t + \epsilon_x\nabla_{X_A^t}\left\{\ell(\theta;X_A^t,Y) - \lambda c_w(X_A^t,X)\right\}\\
	\frac{\partial X_A^{t+1}}{\partial w} &= \frac{\partial X_A^{t}}{\partial w} - 2\epsilon_x\lambda \mathrm{Diag}\left(X_A^t - X\right)\\
	\frac{\partial X_A}{\partial w} &\approx -2\epsilon_x\lambda \sum_t \mathrm{Diag}(X_A^t - X)
\end{align}
which can be accumulated during the adversarial training process.

\subsection{Accuracy}
% 解释一下近似过程
We approximate the $\partial \theta / \partial X_A$ and $\partial X_A / \partial w$ during the gradient descent and ascent process, where we use the average gradient as the approximate value.
% 使用delta R的值来作为梯度估计的评估
We tested the reliability of our approximation empirically.
Since the gradient represents the direction to which the function declines fastest, we compare the $\Delta R$ after updating by our $\partial R / \partial w$ with that after randomly selected directions with the same step size.
The $\Delta R$ brought by the accurate gradient is largest among any other directions.
Therefore, the higher possibility that our $\Delta R$ is larger than randomly picked direction, the more accurate our approximation is.
We perform random experiments for 1000 times, and the approximation of our SAL outperforms 99.4\% of them, which validate the high accuracy of our approximation.

% \subsection{Complexity}
%We induce $\partial R / \partial w$ to find a better covariate weight $w$ for our uncertainty set.
%In this part, we analyze the complexity of the deduction of $\partial R/\partial w$.
%
%
%Consider a 2-layer MLP where $i$ denotes the input size, $j$ the number of nodes in the second layer and $k$ the number of nodes in the output layer. 
%Assume there are $N$ training samples, the computation complexity for single forward pass is $O(N*(ij+jk)*i)$, and the 'mini-batch' version is $O(N_b*(ij+jk)*i)$ with $N_b<<N$ denoting the batch size.
%We run experiments of single hidden layer neural net with 100 neurons and 10 covariates on two CPUs(Intel(R) Xeon(R) CPU E5-2699 v4 @ 2.20GHz).
%The running time for one single pass with $T_{\theta}=100$ and $m=10$ is 180.39s, which is acceptable in terms of time cost.
%
%
%The extra memory cost can be further reduced to $O(N_b*i*(ij+jk))$ with $N_b<<N$ by approximating the $\partial R/\partial w$ to 'mini-batch' version.
%
%Furthermore, the number of iterations $T$ required for the whole algorithm can be significantly reduced by initializing the weight with a better-selected $w$.

\section{Proofs}

\subsection{Proof of Theorem 3.1}
From lemma 2.1, for all $\lambda \geq 0,\ \rho \geq 0$, we have
\begin{equation}
\label{equ:proof1-1}
	\sup\limits_{P:W_{c_w}(P,P_0)}\mathbb{E}_{P}[\ell(\theta;X,Y)]\leq \lambda\rho + \mathbb{E}_{P_0}[s_{\lambda}(\theta;X,Y)]
\end{equation}
Since $-T_{\ell}\leq \ell \leq T_{\ell}$ and $s_{\lambda} = \sup\limits_{z\in \mathcal{Z}}\left\{\ell-\lambda c_w\right\}$, we have:
\begin{equation}
	-T_{\ell}\leq s_{\lambda}\leq T_{\ell}
\end{equation}
Therefore, applying the standard results on Rademacher complexity\cite{bartlett2002rademacher}, with probability at least $1-\delta$, we have:
\begin{align}
	\mathbb{E}_{P_0}[s_{\lambda}] \leq& \\
	&\mathbb{E}_{\hat{P}_n}[s_{\lambda}] + \mathcal{R}_n(\widetilde{l}\circ F) +kT_{\ell}\sqrt{\frac{\ln(1/\delta)}{n}}
\end{align}

And combined with equation \ref{equ:proof1-1}, we have:
\begin{align}
	\sup\limits_{P:W_{c_w}(P,P_0)}&\mathbb{E}_{P}[\ell(\theta;X,Y)]\leq \\
	 &\lambda\rho+ \mathbb{E}_{\hat{P}_n}[s_{\lambda}] + \mathcal{R}_n(\widetilde{l}\circ F) +kT_{\ell}\sqrt{\frac{\ln(1/\delta)}{n}}
\end{align}
Taking $\rho = \hat{\rho}_n$ and lemma 2.1, we have
\begin{align}
	&\sup\limits_{P:W_{c_w}(P,P_0)\leq \hat{\rho}_n(\theta)}\mathbb{E}_P\left[\ell(\theta;Z)\right] =\\
	 &\sup\limits_{P:W_{c_w}(P,\hat{P}_n)\leq \hat{\rho}_n(\theta)} \mathbb{E}_P\left[\ell(\theta;Z)\right] + \mathcal{R}_n(\widetilde{\ell}\circ F) + kT_{\ell}\sqrt{\frac{\ln(1/\delta)}{n}}
\end{align}
where $k$ is a numerical constant no less than 0.

\subsection{Proof of Theorem 3.2}

First, we prove that $\mathcal{P} \subseteq \mathcal{P}_0$. $\forall P \in \mathcal{P}$, there exists measure $M_0$ on $\mathcal{Z}\times\mathcal{Z}$ satisfying:
\begin{equation}
    \mathbb{E}_{(z,z')\sim M_0}[c_w(z,z')] \leq \rho
\end{equation}
Note that $c_w$ is optimal if and only if $min(w^{(i)})=1$ and $max(w^{(i)})>1$. 
Therefore, we have $\forall z,z' \in \mathcal{Z},\ c(z,z') < c_w(z,z')$. Therefore, we have:
\begin{align}
    W_c(P,P_0) &= \mathop{inf}\limits_{M \in \Pi(P,Q)} \mathbb{E}_{(z,z') \sim M}[c(z,z')]\\
    &\leq \mathbb{E}_{(z,z')\sim M_0}[c(z,z')]\\ 
    &< \mathbb{E}_{(z,z')\sim M_0}[c_w(z,z')] \\
    &\leq \rho
\end{align}
and therefore $P \in \mathcal{P}_0$ and $\mathcal{P} \subseteq \mathcal{P}_0$. 

Second, we prove that $\exists Q_0 \in \mathcal{P}_0,\ s.t.\ Q_0 \notin \mathcal{P}$ under assumption 3.1.
We have:
\begin{align}
    \mathbb{E}_{(z,z') \sim M_0}[c_w(z,z')] &> \mathbb{E}_{(z,z') \sim M_0}[c(z,z')] \\
    &\geq \rho
\end{align}
and 
\begin{equation}
    \mathbb{E}_{M \in \Pi(P_0,Q_0)-M_0}[c_w(z,z')] > \rho
\end{equation}

which leverages the property that $\|.\|_1$ and $\|.\|_2^2$ are strictly increasing against the absolute value of each covariate of the independent variable. 

For distribution $Q_0$ satisfying assumption 3.1, we have:
\begin{align}
    \mathbb{E}_{(z,z') \sim M_0}[c_w(z,z')] &> \rho\\
    \mathbb{E}_{M \in \Pi(P_0,Q_0)-M_0}[c_w(z,z')] &> \rho
\end{align}
and therefore:
\begin{equation}
    \mathop{inf}\limits_{M \in \Pi(P,Q)} \mathbb{E}_{(z,z') \sim M}[c_w(z,z')] > \rho
\end{equation}
which proves that $Q_0 \notin \mathcal{P}$. Therefore, we have $\mathcal{P} \subset \mathcal{P}_0$.

Furthermore, we prove that for the set $U = \{i|w^{(i)}=1\},\ \exists Q_0 \in \mathcal{P}$ that satisfies $W_{c_w}(P_{0\#U},Q_{0\#U})=\rho$ with the help of assumption \ref{assump:appendix}. 

\begin{assumption}
\label{assump:appendix}
	Given $\rho\geq 0$ and $c_w$, there exists distribution $V$ supported on $\mathcal{Z}_{\#U}$ that
	\begin{equation}
		W_{c_w}(V, P_{0\#U})=\rho
	\end{equation}
\end{assumption}

Assume that distribution $H$ satisfies assumption \ref{assump:appendix}, we firstly construct a distribution $Q_0$ as following:
\begin{align}
	Q_{0\#U} &= H\\
	\label{equ:proof}
	\forall v \in \mathcal{Z}_{\#U},\ \forall s \in \mathcal{Z}_{\#S}&,\ \ Q_0(s|v) = P_{0\#S}(s)
\end{align}
where $S = \{i|w^{(i)}>1\}$. Since $W_{c_w}(Q_{0\#U}, P_{0\#U}) = \rho$, we have:
\begin{equation}
		\inf_{M \in \Pi(P_{0\#U},Q_{0\#U})} \mathbb{E}_{(z,z') \sim M}[c(z,z')] \leq \rho
\end{equation}
where we refer to the couple minimizing $\mathbb{E}_{(z,z')\sim M_0}[c_w(z,z')]$ as $M_0$. Then we construct joint couple $M$ supported on $\mathcal{Z}\times\mathcal{Z}$, where $M(z,z'),\ z\in\mathcal{Z},\ z'\in\mathcal{Z}$ denotes the probability of transferring $z$ to $z'$. 

Assume $Z=[S,V]$, where $S \in \mathcal{Z}_{\#S}$, $V \in \mathcal{Z}_{\#U}$. $\forall v_1,v_2 \in \mathcal{Z}_{\#U}$, according to equation \ref{equ:proof}, distribution $P_0(S|V=v_1)$ is the same as $Q_0(S|V=v_2)$ and the optimal transportation cost between them is zero. 

For some transportation scheme $\hat{M}$ on $\mathcal{Z}\times\mathcal{Z}$, 
\begin{align}
		&\int_{z \in \mathcal{Z}}\int_{z' \in \mathcal{Z}}c_w(z,z')\hat{M}(z,z') dz dz'\\
		=& \int_{v \in \mathcal{Z}_{\#U}}\int_{v' \in \mathcal{Z}_{\#U}} dv dv' \\
		&\left\{  \int_{s \in \mathcal{Z}_{\#S}}\int_{s' \in \mathcal{Z}_{\#S}} c_w([s,v],[s',v'])\hat{M}([s,v],[s',v']) ds ds' \right\}\\
		\label{equ:mstar}
		=& \int_{v \in \mathcal{Z}_{\#U}}\int_{v' \in \mathcal{Z}_{\#U}} c_w(v,v')\hat{M}^*(v,v')dvdv'
\end{align}
$\hat{M}^*$ in equation \ref{equ:mstar} denotes the distribution on $\mathcal{Z}_{\#U}\times\mathcal{Z}_{\#U}$. 
Therefore, we have
\begin{align}
		&W_{c_w}(P_0,Q_0) \\
		&= \inf_{M \in \Pi(P_0,Q_0)} \int_{z \in \mathcal{Z}}\int_{z' \in \mathcal{Z}}c_w(z,z')M(z,z') dz dz'\\
		&= \inf_{M \in \Pi(P_{0\#U},Q_{0\#U})}\int_{v \in \mathcal{Z}_{\#U}}\int_{v' \in \mathcal{Z}_{\#U}} c_w(v,v')M(v,v')dvdv'\\
		&= W_{c_w}(P_{0\#U}, Q_{0\#U})\\
		&= \rho 
\end{align}

\section{Experimental Details}
Due to the space limitations, we have omitted some experimental details in the main body, which are introduced here. 

\subsection{Details of Toy Example}
The goal is to predict $y \in \mathcal{R}$ from $x \in \mathcal{R}^d$, and we use $\ell(\theta;(x,y)) = |y - \theta^Tx|$ as the loss function. 
In this case, we take $d=2$ and generate $X = [S,V]^T$, where $S\stackrel{iid}{\sim} \mathcal{N}(0,0.5)$. We then generate $Y$ and $V$ as following:
\begin{align}
	Y &= 5*S + S^2 + \epsilon_1 \\
	V &= \alpha Y + \epsilon_2 
\end{align}
where $\epsilon_1 \stackrel{iid}{\sim} \mathcal{N}(0,0.1)$ and $\epsilon_2 \stackrel{iid}{\sim} \mathcal{N}(0,1.0)$.

In training, we generate 180 data points from environment 1 with $\alpha=1.0$ and 20 data points from environment 2 with $\alpha=-1.0$. 
In testing, we compared methods across environments with $\alpha\in\{-2.0,-1.9,\dots,1.9,2.0\}$. 
The results are shown in figure \ref{img:toy-app}, where we add the results of IRM.
We select the hyper-parameter $\lambda$ in $\{1e-3,1e-2,2e-2,\dots,1e-1,\dots,1.0\}$ and select the best one according to the validation data which are sampled i.i.d from training environments.  
In this experiment, we find that IRM has the worst performance, which we think is due to the high demands that IRM requires for the discrepancy of training environments.
Although this example is simple, it can strongly suggest that our method is effective since there is no other interference factors.

\begin{figure}
	\centering
	\includegraphics[width=0.9\linewidth]{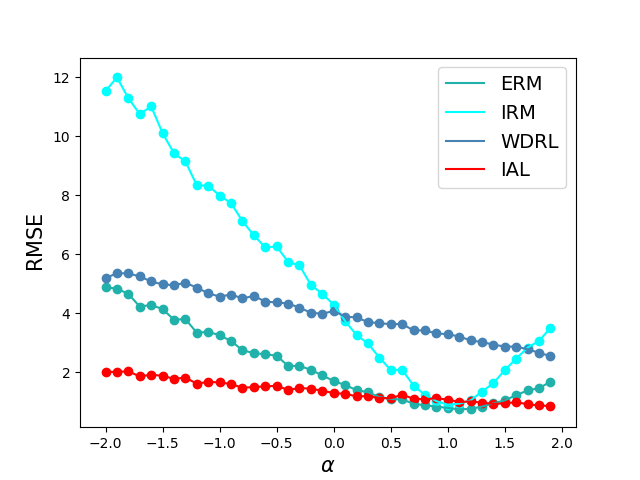}
	\caption{Results of the toy example.}
	\label{img:toy-app}
\end{figure}

\subsection{Details of Selection Bias}
In this setting, we assume $X = [S,V]^T \in \mathcal{R}^p$ and $S = [S_1, S_2, \dots, S_{n_s}]^T \in \mathcal{R}^{n_s}$ is independent from $V = [V_1, V_2, \dots, V_{n_v}]\in \mathcal{R}^{n_v}$ while the covariates in $S$ are dependent with each other. 
Therefore, we generate training data points with the help of auxiliary variables $Z \in \mathcal{R}^d$ as following:
\begin{align}
Z_1, \dots, Z_d &\stackrel{iid}{\sim} \mathcal{N}(0,1.0) \\
V_1, \dots, V_{n_v} &\stackrel{iid}{\sim} \mathcal{N}(0,1.0) \\
S_i = 0.8*Z_i + 0.2 * Z_{i+1} &\ \ \ \ \ for \ \ i = 1, \dots, n_s
\end{align}
To induce model misspecification, we generate $Y$ as:
\begin{equation}
Y = f(S) + \epsilon = \theta_s*S^T + \beta*S_1S_2S_3+\epsilon
\end{equation}
where $\theta_s = [\frac{1}{3},-\frac{2}{3}, 1, -\frac{1}{3}, \frac{2}{3}, -1 , \dots] \in \mathcal{R}^{n_s}$, and $\epsilon \sim \mathcal{N}(0, 0.3)$. 
We assume that $P(Y|S)$ remains unchanged while $P(Y|V)$ can vary across environments. 
Here we design a data selection mechanism to induce this kind of distribution shifts.
For simplicity, we select data points according to a certain variable $v_i \in V$:

\begin{align}
&\hat{P} = |r|^{-5*|f(s) - sign(r)*v_i|}  \\
&\mu \sim Uni(0,1 ) \\
&M(r;(x,y)) =
\begin{cases}
1, \ \ \ \ \ &\text{$\mu \leq \hat{P}$ } \\
0, \ \ \ \ \ &\text{otherwise}
\end{cases} 
\end{align}  
where $|r| > 1$.
Given a certain $r$, a data point $(x,y)$ is selected if and only if $M(r;(x,y))=1$ (i.e. if $r>0$, a data point whose $v_i$ is close to its $y$ is more probably to be selected.)

In this setting, we take $d=10$ and $n_s = n_v = 5$.  
In the training, we generate $n$ data points, where $\kappa n$ points form environment $e1$ with a predefined $r$ and $(1-\kappa)n$ data points form environment $e2$ with $r=-1.1$. 
In the testing, we generate test data points for 10 environments with $r \in [-3,-2,-1.7,-1.5,-1.3,1.3,1.5,1.7,2,3]$.

\subsection{Details of Anti-Causal Effect}
In this setting, we introduce the spurious correlation by using anti-causal relationship from the target $Y$ to the unstable covariates $V$.
We assume $X=[S,V]^T \in \mathcal{R}^m$ and $S = [S_1, \dots, S_{n_s}]^T\in \mathcal{R}^{n_s}$, $V=[V_1, \dots, V_{n_v}]^T\in \mathcal{R}^{n_v}$. 
Data Generation process is as following:
\begin{align}
	S &\sim \sum_{i=1}^k z_k \mathcal{N}(\mu_i,I)\\
	Y &= \theta_s^TS + \beta S_1S_2S_3+\mathcal{N}(0,0.3)\\
	V &= \theta_v Y + \mathcal{N}(0,\sigma(\mu_i)^2)
\end{align}  
where $\sum_{i=1}^k z_i = 1\ \&\  z_i >= 0$ is the mixture weight of $k$ Gaussian components, $\sigma(\mu_i)$ means the Gaussian noise added to $V$ depends on which component the stable covariates $S$ belong to and $\theta_v \in \mathcal{R}^{n_v}$. 

We use the mixture weight $Z=[z_1,\dots,z_k]^T$ to define different environments, where different mixture weights represent different overall strength of the effect $Y$ on $V$.

In this experiment, we set $n_s=n_v=5$, $k=10$, $\mu_1=[0,0,0,1,1]^T,\mu_2 = [0,0,0,1,-1]^T,\mu_2=[0,0,0,-1,1]^T,\mu_4=\mu_5=\dots=\mu_{10}=[0,0,0,-1,-1]^T$, $\sigma(\mu_1)=0.2, \sigma(\mu_2)=0.5,\sigma(\mu_3)=1.0$ and $[\sigma(\mu_4), \sigma(\mu_5),\dots,\sigma(\mu_{10})]=[3.0,5.0,\dots,15.0]$. 
$\theta_s, \theta_v$ are randomly sampled from $\mathcal{N}(1,I_5)$ and $\mathcal{N}(0,0.1I_5)$ respectively in each run, we run experiments for 15 times and average the results. 

In the training, data points come from three environments including 1000 points from $e_1$ with $Z=[1,0,\dots,0]$, 100 points from $e_2$ with $Z=[0,1,0,\dots,0]$ and 100 points from $e_3$ with $Z=[0,0,1,0,\dots,0]^T$. 
Note that the last seven components are not captured by the training data, and we mainly use these components for testing.

\subsection{Details of Classification}
\subsubsection{Colored MNIST}

In this task, we build a synthetic binary classification task derived from MNIST. 
We color each image either red or green in a way that strongly correlates with the class label, which is spurious correlation.
Firstly, we assign each image a binary label $y$ based on the label: $y=0$ for digits $0 \sim 4$ and $y=1$ for $5\sim 9$.
Secondly, we sample the color id $z$ by flipping $y$ with probability $\mu$, where $\mu$ is 0.0 for environment 1, 0.3 for the second and 1.0 for testing.
Thirdly, we induce noisy label by randomly flipping the label $y$ with probability 0.2.
In the training, we consider the imbalanced setting which is more challenging and practical.
Specifically, we sample 20,000 images from environment 1 and 500 from 2 as training data and 10,000 from testing environment.
It is reasonable to assume that models optimized by empirical risk minimization will fail under the influence of spurious correlations(color).

% 不同baseline方法
For ERM, we pool all data together and train a CNN model end-to-end.
For IRM, we use the same architecture and optimize it using the loss function proposed in \cite{arjovsky2019invariant}.
For DRL methods, we first use the unsupervised method proposed in \cite{2018Unsupervised} to extract features of 128 dimensions, and the model used has the same architecture as above.
Then we perform WDRL and our SAL using the extracted features as input.
The architecture of the model includes 3 CNN layers with output channels 16, 64, 128 respectively and 2 FC layers with output neurons 512, 128 and we use ReLU for activation.

% 测试方法和验证方法
For all methods, we select the hyper-parameters according to the performance on the validation set.
We sample 1000 data from the two training environments respectively and select the hyper-parameters which maximize the minimum accuracy of two validation environments.
Note that we have no access to the testing environment while training, therefore we cannot resort to testing data to select the best one, which is more reasonable and different from \cite{arjovsky2019invariant}.

\section{Explanations for the confidence}
To better illustrate the low confidence problem, we design a simulated classification experiment.

\section{Additional empirical results}
In this section, we give more experimental results. 

\subsection{More Baselines}
Firstly, we add two baselines:
\begin{itemize}
	\item LASSO: 
		\begin{equation}
			\min_{\theta}\mathbb{E}_{p_0}[\ell(\theta;X,Y)] + \lambda \|\theta\|_1
		\end{equation}
	\item Ridge:
		\begin{equation}
			\min_{\theta}\mathbb{E}_{p_0}[\ell(\theta;X,Y)] + \lambda \|\theta\|_2^2
		\end{equation}
\end{itemize} 

In experiments, we search the hyper-parameters $\lambda$ for LASSO and Ridge in $\{1e-3, 1e-2, \dots, 1e-1, \dots, 1e0,1e1\}$ and select the best one according to the validation set.
The validation data are sampled i.i.d from the training environments.

Then we introduce one more baseline according to \cite{blanchet2019data} for our simulation datasets, which uses metric learning methods to learn a transportation cost function for WDRL. 
However, the starting point of our methods are totally different and their method does not involve covariate's differentiation as well as one solution to the over-pessimism problem for WDRL. 
Furthermore, their method contains two separate blocks, metric learning and robust optimization, while in our method the process of learning the transportation cost function and the process of optimization model's parameters are united. 
For completeness, we consider this method as an extra baseline in our supplementary experiments. 

In our experiments, in order to adapt the regression scenarios, we split the training data into ten groups according to the value of $Y$ and perform metric learning methods. 
Specifically, we use Neighbourhood Components Analysis\cite{goldberger2005neighbourhood} for learning the cost function, and the method is referred to as MDRL in the following.

\subsection{Selection Bias}
As for the selection bias simulation experiment in the main body, for simplicity, the dimension of unstable covariates is one. 
Here we give a more general setting with multiple unstable covariates. 

The corresponding data generation process becomes:
\begin{align}
&\hat{P} = \Pi_{v_i \in V} |r_i|^{-5*|f(s) - sign(r_i)*v_i|}  \\
&\mu \sim Uni(0,1 ) \\
&M(r;(x,y)) =
\begin{cases}
1, \ \ \ \ \ &\text{$\mu \leq \hat{P}$ } \\
0, \ \ \ \ \ &\text{otherwise}
\end{cases} 
\end{align}  
where $r = [r_1, \dots, r_{n_{b}}]^T$ and $|r_i| > 1$, $n_b$ denotes the number of dimensions to be applied the selection bias. 

In this setting, we take $d=10$ and $n_s = n_v = 5$, and we apply selection bias on the last three dimension of the unstable covariate $V$ ($n_b=3$). 
In the training, we generate $n$ data points, where $\kappa n$ points form environment $e1$ with a predefined $r=[2.0,1.7,1.5]$ and $(1-\kappa)n$ data points form environment $e2$ with $r=[-1.1,-1.1,-1.1]$. 
In the testing, we generate test data points for 10 environments with $r_1 \in [-3,-2.5,-2,-1.7,-1.5,1.5,1.7,2,2.5,3]$ and $r = [r_1, 0.9*r_1, 0.8*r_1]$. 

% results 
\begin{table*}[htbp]
	\centering
	\caption{Results of the selection bias experiment.}
	\label{tab:supplementary1}
	\vskip 0.05in
	
%	\resizebox{\textwidth}{15mm}{
	\begin{tabular}{|l|c|c|c|c|c|c|}
		\hline
		\multicolumn{7}{|c|}{\textbf{Scenario 1: varying selection bias rate $r$\quad($n=2000,p=10,\kappa=0.95$)}}\\
		\hline
		$r$&\multicolumn{2}{|c|}{$r=1.5$}&\multicolumn{2}{|c|}{$r=1.7$}&\multicolumn{2}{|c|}{$r=2.0$}\\
		\hline
		Methods &  $Mean\_Error$ & $Std\_Error$ &$Mean\_Error$ & $Std\_Error$ &  $Mean\_Error$ & $Std\_Error$  \\
		\hline % setting 1
		ERM & 0.484 & 0.058 & 0.561 & 0.124  & 0.572 & 0.140  \\
		LASSO&0.482 & 0.046 & 0.561 & 0.124  & 0.572 & 0.140\\
		Ridge& 0.483&0.045 & 0.560 & 0.125 & 0.572 & 0.140\\
		WDRL& 0.482 & 0.044& 0.550 & 0.114  & 0.532 & 0.112 \\
		IRM & 0.494 & 0.083 & 0.537 & 0.133 & 0.596 & 0.191 \\
		\hline
		SAL &\bf 0.450 &\bf 0.019 &\bf  0.449 &\bf  0.015  &\bf 0.452 &\bf 0.017 \\
		\hline
		\multicolumn{7}{|c|}{\textbf{Scenario 2: varying ratio $\kappa$ and sample size $n$\quad($p=10,r = 1.7$)}}\\
		\hline
		$\kappa,n$&\multicolumn{2}{|c|}{$\kappa=0.90, n=500$}&\multicolumn{2}{|c|}{$\kappa=0.90, n=1000$}&\multicolumn{2}{|c|}{$\kappa=0.975, n=4000$}\\
		\hline
		Methods &$Mean\_Error$ & $Std\_Error$ &$Mean\_Error$ & $Std\_Error$ &   $Mean\_Error$ & $Std\_Error$ \\
		\hline % 
		ERM & 0.580 & 0.103 & 0.562 & 0.113  & 0.555 & 0.110 \\ 
		LASSO&0.562 & 0.110 & 0.514 & 0.078  & 0.555 & 0.122\\
		Ridge&0.561 & 0.107 & 0.517 & 0.080  & 0.555 & 0.121\\
		WDRL & 0.563 & 0.101& 0.527 & 0.083 & 0.536 & 0.108 \\
		IRM & 0.545 & 0.136 & 0.539 & 0.134 & 0.535	& 0.129\\
		\hline
		SAL &\bf 0.454 & \bf 0.015 & \bf 0.451 & \bf 0.015 & \bf 0.448 & \bf 0.014\\
		\hline

		\multicolumn{7}{|c|}{\textbf{Scenario 3: varying ratio $\kappa$ and sample size $n$($p=10$, $r=2.0$, $n_b=3$)}}\\
		\hline
		$r$&\multicolumn{2}{|c|}{$n=1000,\kappa=0.9$}&\multicolumn{2}{|c|}{$n=2000,\kappa=0.95$}&\multicolumn{2}{|c|}{$n=4000,\kappa=0.975$}\\
		\hline
		Methods &  $Mean\_Error$ & $Std\_Error$ &$Mean\_Error$ & $Std\_Error$ &  $Mean\_Error$ & $Std\_Error$  \\
		\hline % setting 1
		ERM & 0.440 & 0.069 & 0.466 & 0.105  & 0.489 & 0.133  \\
		LASSO&0.433 & 0.059 & 0.460 & 0.097  & 0.482 & 0.124\\
		Ridge&0.434 & 0.061 & 0.457 & 0.095 & 0.481 & 0.124\\
		IRM & 0.528 & 0.161 & 0.526 & 0.161 & 0.528 & 0.164 \\
		WDRL& 0.433 & 0.058 & 0.459 & 0.095  & 0.481 & 0.122 \\
		MDRL& 0.451	& 0.077	& 0.480	& 0.113 	 &  	0.510 & 0.146 \\    
		\hline
		SAL &\bf 0.415 &\bf 0.019 &\bf  0.411 &\bf  0.015  &\bf 0.411 &\bf 0.016 \\
		\hline
	\end{tabular}
%	}
% 	\vskip -0.05in
\end{table*}

From the results shown in table \ref{tab:supplementary1}, our SAL method significantly outperforms all baselines including the extra baselines MDRL, LASSO and Ridge, which further validates the effectiveness of our method.

\subsection{Anti-Causal Effect}
% TODO add results for (S=5,V=5;S=9,V=1)
\begin{table*}[htbp]
	\centering
	\caption{Results of anti-causal effect.}
	\label{tab:supplementary2}
	\vskip 0.05in
	
%	\resizebox{\textwidth}{30mm}{
	\begin{tabular}{|l|c|c|c|c|c|c|c|c|c|c|}
		\hline
		\multicolumn{11}{|c|}{\textbf{Scenario 1: $n_s=5,\ n_v=5$}}\\
		\hline
		$e$&\multicolumn{3}{|c|}{Training environments}&\multicolumn{7}{|c|}{Testing environments}\\
		\hline
		Methods &  $e_1$ & $e_2$ &$e_3$ & $e_4$ &  $e_5$ & $e_6$ &$e_7$ & $e_8$  & $e_9$ & $e_{10}$  \\
		\hline % setting 1
		ERM & 0.2807 & 0.3051 & 0.3409 & 0.4612 & 0.5549 & 0.6362& 0.7029& 0.7327 & 0.7651 & 0.8237  \\
		LASSO& 0.2767& 0.3047 & 0.3414 & 0.4698 & 0.5685 & 0.6484& 0.7222& 0.7520 & 0.7953 & 0.8428\\
		Ridge& \bf 0.2579& 0.3064 & 0.3465 & 0.4833 & 0.5884 & 0.6730& 0.7509& 0.7828 & 0.8278 & 0.8786\\
		IRM & 0.2855 &\bf 0.3043 & 0.3338 & 0.4346 & 0.5139 & 0.5848 & 0.6382 & 0.6675 & 0.6953 & 0.7436 \\
		WDRL&0.2818 & 0.3307 & 0.3986 & 0.5993 & 0.7498 & 0.8750 & 0.9828 & 1.0295 & 1.0719 & 1.1645 \\
		MDRL& 0.2756 & 0.3100 & 0.3597 & 0.8425 & 0.5126 &
       0.6265 & 0.7272 & 0.8076 & 0.8861 & 0.9543 \\   
		\hline
		SAL &0.3244 & 0.3289 &\bf 0.3311 &\bf  0.3577 &\bf 0.3807 & \bf 0.4032 &\bf 0.4246 &\bf 0.4353 &\bf 0.4456 &\bf 0.4575 \\
		\hline
		
		\multicolumn{11}{|c|}{\textbf{Scenario 2: $n_s=9,\ n_v=1$}}\\
		\hline
		$e$&\multicolumn{3}{|c|}{Training environments}&\multicolumn{7}{|c|}{Testing environments}\\
		\hline
		Methods &  $e_1$ & $e_2$ &$e_3$ & $e_4$ &  $e_5$ & $e_6$ &$e_7$ & $e_8$  & $e_9$ & $e_{10}$  \\
		\hline % setting 1
		ERM &\bf 0.2721 &  0.2798 & 0.2983 & 0.5258 & 0.3615 & 0.4110 &
  0.4595 &  0.5042 &  0.5337 &  0.5800  \\
  		LASSO& 0.3094 & 0.3124 & 0.3272 & 0.3602& 0.3968 & 0.4245& 0.4569  & 0.4606 & 0.4729 & 0.4944\\
		Ridge&0.3093 & 0.3133 & 0.3294 & 0.3673 & 0.4079 & 0.4390& 0.4741  & 0.4791 & 0.4932 & 0.5167\\
		IRM & 0.2760 &\bf  0.2797 & 0.2947 & 0.4769 & 0.3438 & 0.3822 &  0.4203 & 0.4588 &  0.4814 & 0.5242 \\
		WDRL&0.2998 & 0.3138 & 0.3317 & 0.5447 & 0.3956 & 0.4405 &
  0.4826 &  0.5287 &0.5547 &0.5963 \\
		MDRL&0.2999 & 0.3201 &   0.3451 & 0.6175 &  0.4300 & 0.4882 &
  0.5425 &  0.5984 & 0.6306 &  0.6803 \\   
		\hline
		SAL &0.2899 & 0.2843 &\bf 0.2876 &\bf 0.2932 &\bf 0.2865 &\bf 0.2884 &\bf
  0.2872 &\bf  0.2900 &\bf 0.2842 &\bf  0.2940 \\
		\hline
	\end{tabular}
%	}
% 	\vskip -0.05in
\end{table*}
We add the results of LASSO and Ridge in Table \ref{tab:supplementary2}.
Results in Table \ref{tab:supplementary2} further validate the effectiveness of our proposed method SAL.

\begin{figure*}[!ht]
\small
\vskip -0.1in
     \begin{minipage}{0.65\textwidth}
       \subfigure[$Mean\_Error$ and $Std\_Error$.]{\label{img:house-summary_app}\includegraphics[width=0.49\textwidth]{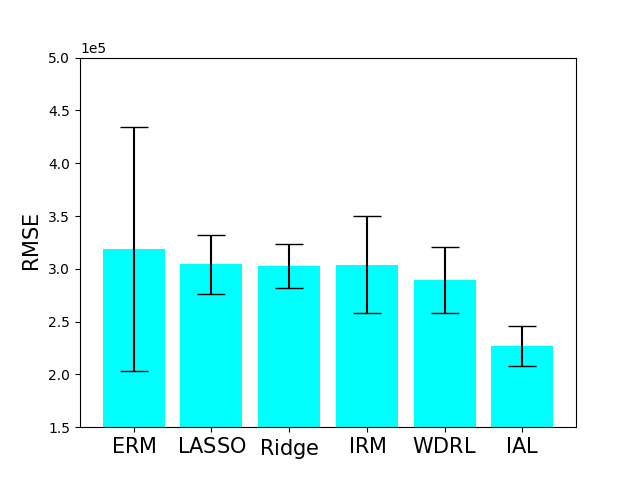}}
       \hfill
		\subfigure[Prediction error with respect to build year.]{\label{img:house-month_app}\includegraphics[width=0.49\textwidth]{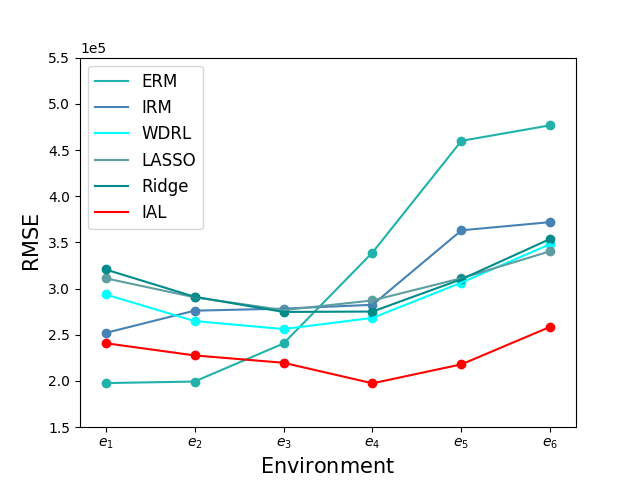}}       
		\caption{Results of the real regression dataset.}
     \end{minipage}
     \hfill
     \begin{minipage}{0.35\textwidth}
     
       \includegraphics[width=\textwidth]{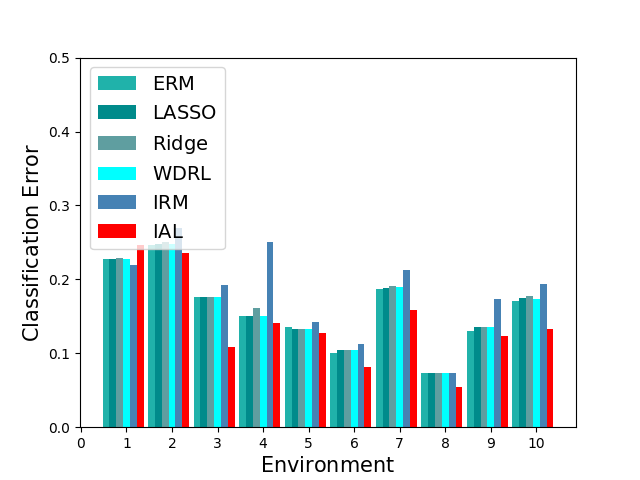}
       \caption{Results of the Adult dataset.}
       \label{img:adults_app}
     \end{minipage}
     \vskip -0.1in
\end{figure*}

\subsection{House Price Prediction}
Figure \ref{img:house-summary_app} and \ref{img:house-month_app} show the results of our real world regression experiment and we add the results of LASSO and Ridge.
We can see that our SAL outperforms all baselines significantly with respect to the uniformly good performance across environments, which validates the effectiveness of our proposed method.
And the results also suggest that there exist distributional shifts across different periods.

\subsection{Income Prediction}
Figure \ref{img:adults_app} shows the results of our real world classification experiment, which further validates the effectiveness of our method.
